# Supplementary material for: Rotated Robustness: A Training-Free Defense against Bit-Flip Attacks on Large Language Models
Source: arXiv:2603.16382 source file (2026-11-10)
Supplement: Supplementary file 1 [file appendix.tex]

% ==========================================
% Appendices
% ==========================================
\appendices

% =================================================
% Appendix: RQ2 完整PBS结果
% =================================================
\subsection{Complete Gray-Box PBS Results}
\label{appendix:pbs_full}

Table~\ref{tab:rq2_pbs_full} reports the complete numerical summary for RQ2. ``First $K$'' denotes the first cumulative PBS bit count at which PPL exceeds 100; $>100$ indicates that no threshold crossing occurs within PBS100.

\begin{table*}[t]
    \centering
    \caption{Complete gray-box PBS results across eight models. ``First $K$'' denotes the first cumulative PBS bit count at which PPL exceeds 100; $>100$ indicates no threshold crossing within PBS100.}
    \label{tab:rq2_pbs_full}
    \scriptsize
    \resizebox{\textwidth}{!}{%
    \begin{tabular}{llcccccc}
        \toprule
        \textbf{Model} & \textbf{Method}
        & \textbf{Clean PPL}
        & \textbf{First $K$}
        & \textbf{PPL@20}
        & \textbf{PPL@50}
        & \textbf{PPL@100}
        & \textbf{Max PPL} \\
        \midrule
        \multirow{5}{*}{OPT-125M} & Baseline & 25.17 & 3 & $1.14{\times}10^{4}$ & $9.40{\times}10^{5}$ & $5.82{\times}10^{4}$ & $1.38{\times}10^{6}$ \\
         & FaR & 26.01 & 3 & $5.69{\times}10^{3}$ & $8.58{\times}10^{3}$ & $2.89{\times}10^{5}$ & $3.05{\times}10^{5}$ \\
         & RADAR & 25.17 & 3 & 564.24 & $3.90{\times}10^{3}$ & $4.27{\times}10^{3}$ & $4.27{\times}10^{3}$ \\
         & QuaRot-Had & 25.27 & 40 & 40.48 & 243.85 & $1.13{\times}10^{4}$ & $1.13{\times}10^{4}$ \\
         & \textbf{RoR (Ours)} & 25.18 & 79 & 33.69 & 64.84 & 139.35 & 139.35 \\
        \midrule
        \multirow{5}{*}{SmolLM2-360M} & Baseline & 11.05 & 3 & $4.52{\times}10^{10}$ & $2.45{\times}10^{39}$ & $1.89{\times}10^{68}$ & $1.89{\times}10^{68}$ \\
         & FaR & 15.93 & 7 & $7.01{\times}10^{4}$ & $2.52{\times}10^{14}$ & $2.46{\times}10^{27}$ & $2.46{\times}10^{27}$ \\
         & RADAR & 11.05 & 10 & $6.31{\times}10^{3}$ & $1.56{\times}10^{4}$ & $8.19{\times}10^{4}$ & $3.28{\times}10^{6}$ \\
         & QuaRot-Had & 11.05 & 43 & 19.40 & 186.88 & $2.37{\times}10^{4}$ & $2.37{\times}10^{4}$ \\
         & \textbf{RoR (Ours)} & 11.05 & $>100$ & 11.07 & 11.07 & 32.97 & 32.97 \\
        \midrule
        \multirow{5}{*}{Qwen2.5-0.5B} & Baseline & 12.52 & 4 & $5.91{\times}10^{11}$ & $9.30{\times}10^{23}$ & $3.96{\times}10^{30}$ & $3.96{\times}10^{31}$ \\
         & FaR & 53.53 & 3 & $6.41{\times}10^{10}$ & $4.87{\times}10^{16}$ & $8.60{\times}10^{21}$ & $6.52{\times}10^{23}$ \\
         & RADAR & 12.52 & 46 & 25.68 & 104.21 & $1.49{\times}10^{6}$ & $1.49{\times}10^{6}$ \\
         & QuaRot-Had & 12.50 & 80 & 13.12 & 14.15 & $7.23{\times}10^{3}$ & $7.23{\times}10^{3}$ \\
         & \textbf{RoR (Ours)} & 12.52 & 99 & 13.01 & 16.23 & 111.10 & 111.10 \\
        \midrule
        \multirow{5}{*}{Llama-3.2-1B} & Baseline & 9.08 & 6 & $9.99{\times}10^{3}$ & $2.29{\times}10^{5}$ & $2.66{\times}10^{5}$ & $7.34{\times}10^{7}$ \\
         & FaR & 13.81 & 12 & $6.50{\times}10^{3}$ & $1.55{\times}10^{18}$ & $4.24{\times}10^{19}$ & $7.14{\times}10^{19}$ \\
         & RADAR & 9.08 & 30 & 10.01 & $2.95{\times}10^{4}$ & 118.63 & $7.79{\times}10^{4}$ \\
         & QuaRot-Had & 9.06 & $>100$ & 9.07 & 9.09 & 9.13 & 9.13 \\
         & \textbf{RoR (Ours)} & 9.07 & $>100$ & 9.20 & 9.54 & 9.94 & 9.94 \\
        \midrule
        \multirow{5}{*}{Llama-2-7B} & Baseline & 5.18 & 3 & $2.25{\times}10^{5}$ & $2.26{\times}10^{7}$ & $2.28{\times}10^{38}$ & $6.20{\times}10^{39}$ \\
         & FaR & 7.99 & 14 & $1.09{\times}10^{4}$ & $2.10{\times}10^{6}$ & $3.08{\times}10^{35}$ & $3.08{\times}10^{35}$ \\
         & RADAR & 5.18 & 7 & $9.18{\times}10^{3}$ & $1.11{\times}10^{4}$ & $1.76{\times}10^{4}$ & $1.78{\times}10^{4}$ \\
         & QuaRot-Had & 5.18 & $>100$ & 5.19 & 5.23 & 5.32 & 5.32 \\
         & \textbf{RoR (Ours)} & 5.18 & $>100$ & 5.19 & 5.23 & 5.31 & 5.31 \\
        \midrule
        \multirow{5}{*}{Qwen2.5-7B} & Baseline & 6.13 & 18 & $1.01{\times}10^{3}$ & $3.47{\times}10^{8}$ & $5.99{\times}10^{24}$ & $6.93{\times}10^{37}$ \\
         & FaR & 8.39 & 46 & 13.19 & 263.48 & $7.04{\times}10^{9}$ & $7.04{\times}10^{9}$ \\
         & RADAR & 6.13 & 86 & 8.20 & 21.33 & 611.73 & 611.73 \\
         & QuaRot-Had & 6.13 & $>100$ & 6.17 & 6.23 & 6.45 & 6.45 \\
         & \textbf{RoR (Ours)} & 6.12 & $>100$ & 6.20 & 6.35 & 6.84 & 6.84 \\
        \midrule
        \multirow{5}{*}{Qwen2.5-14B} & Baseline & 4.45 & 12 & $4.92{\times}10^{4}$ & $3.56{\times}10^{8}$ & $1.79{\times}10^{11}$ & $2.02{\times}10^{13}$ \\
         & FaR & 5.43 & 27 & 10.25 & $9.69{\times}10^{3}$ & $9.43{\times}10^{4}$ & $9.99{\times}10^{4}$ \\
         & RADAR & 4.45 & 93 & 4.59 & 4.98 & $2.78{\times}10^{4}$ & $2.78{\times}10^{4}$ \\
         & QuaRot-Had & 4.44 & $>100$ & 4.47 & 4.50 & 4.63 & 4.63 \\
         & \textbf{RoR (Ours)} & 4.45 & $>100$ & 4.47 & 4.52 & 4.75 & 4.75 \\
        \midrule
        \multirow{5}{*}{Mistral-Nemo-Base-2407} & Baseline & 5.28 & 2 & $1.16{\times}10^{14}$ & $3.65{\times}10^{10}$ & $2.68{\times}10^{24}$ & $2.68{\times}10^{24}$ \\
         & FaR & 7.67 & 36 & 16.17 & $1.15{\times}10^{3}$ & $1.27{\times}10^{8}$ & $1.27{\times}10^{8}$ \\
         & RADAR & 5.28 & 18 & $4.66{\times}10^{5}$ & 96.57 & $3.11{\times}10^{5}$ & $7.42{\times}10^{7}$ \\
         & QuaRot-Had & 5.29 & $>100$ & 5.31 & 5.32 & 5.33 & 5.33 \\
         & \textbf{RoR (Ours)} & 5.28 & $>100$ & 5.31 & 5.31 & 5.32 & 5.32 \\
        \bottomrule
    \end{tabular}%
    }
\end{table*}






% =================================================
% Appendix: RQ4 三模型 PBS100 下游任务结果
% =================================================
\subsection{Additional Downstream-Task Results}
\label{appendix:rq4_full}

For completeness, Table~\ref{tab:rq4_ci_full} reports PBS100 downstream-task accuracy for Llama-3.2-1B, Llama-2-7B, and Qwen2.5-7B. Brackets denote two-sided 95\% Wilson confidence intervals computed from the fixed evaluation subsets.

\begin{table*}[t]
    \centering
    \caption{Downstream-task accuracy at PBS100 across three evaluated models. Each entry reports accuracy (\%) followed by its two-sided 95\% Wilson confidence interval. The four-domain MMLU subset contains 400 evaluated examples; HellaSwag and PIQA contain 100 examples each.}
    \label{tab:rq4_ci_full}
    \scriptsize
    \resizebox{\textwidth}{!}{%
    \begin{tabular}{llccc}
        \toprule
        \textbf{Model} & \textbf{Method}
        & \textbf{MMLU subset}
        & \textbf{HellaSwag}
        & \textbf{PIQA} \\
        \midrule
        \multirow{5}{*}{Llama-3.2-1B} & Baseline & 20.75 [17.06, 24.99] & 25.00 [17.55, 34.30] & 55.00 [45.24, 64.39] \\
         & FaR & 29.50 [25.24, 34.15] & 31.00 [22.78, 40.63] & 56.00 [46.23, 65.33] \\
         & RADAR & 24.50 [20.54, 28.94] & 43.00 [33.73, 52.78] & 56.00 [46.23, 65.33] \\
         & QuaRot-Had & 29.25 [25.01, 33.89] & 62.00 [52.21, 70.90] & 80.00 [71.12, 86.66] \\
         & \textbf{RoR (Ours)} & 28.25 [24.06, 32.85] & 61.00 [51.20, 69.98] & 81.00 [72.22, 87.49] \\
        \midrule
        \multirow{5}{*}{Llama-2-7B} & Baseline & 26.75 [22.65, 31.29] & 35.00 [26.36, 44.75] & 52.00 [42.32, 61.54] \\
         & FaR & 22.75 [18.91, 27.11] & 36.00 [27.27, 45.76] & 54.00 [44.26, 63.44] \\
         & RADAR & 22.75 [18.91, 27.11] & 30.00 [21.89, 39.58] & 52.00 [42.32, 61.54] \\
         & QuaRot-Had & 44.00 [39.22, 48.90] & 72.00 [62.51, 79.86] & 77.00 [67.85, 84.16] \\
         & \textbf{RoR (Ours)} & 44.25 [39.46, 49.15] & 73.00 [63.57, 80.73] & 78.00 [68.93, 85.00] \\
        \midrule
        \multirow{5}{*}{Qwen2.5-7B} & Baseline & 22.75 [18.91, 27.11] & 25.00 [17.55, 34.30] & 58.00 [48.21, 67.20] \\
         & FaR & 58.75 [53.86, 63.47] & 45.00 [35.61, 54.76] & 67.00 [57.31, 75.44] \\
         & RADAR & 69.00 [64.30, 73.33] & 57.00 [47.22, 66.27] & 74.00 [64.63, 81.60] \\
         & QuaRot-Had & 71.25 [66.63, 75.47] & 73.00 [63.57, 80.73] & 85.00 [76.72, 90.69] \\
         & \textbf{RoR (Ours)} & 71.50 [66.89, 75.70] & 72.00 [62.51, 79.86] & 84.00 [75.58, 89.90] \\
        \bottomrule
    \end{tabular}%
    }
\end{table*}
